# Supplementary material for: First-principles study of inter-site magnetic couplings and Curie temperature in RFe$_{12-x}$Cr$_{x}$ (R = Y, Nd, Sm)
Source: arXiv:1711.05137 ancillary file (2018-01-17)
Supplement: Supplementary file 1 [file nasu_suppl.pdf]

# Supplemental material to “First-principles study of intersite magnetic couplings and Curie temperature in $RFe_{12-x}Cr_x$ (R = Y, Nd, Sm)”

Taro Fukazawa[1,3], Hisazumi Akai[2,3], Yosuke Harashima[1,3] and Takashi Miyake[1,31]

[1]CD-FMat, National Institute of Advanced Industrial Science and Technology, Tsukuba, Ibaraki 305-8568, Japan
[2]The Institute for Solid State Physics, The University of Tokyo, 5-1-5 Kashiwano-ha, Kashiwa, Chiba 277-8581, Japan
[3]ESICMM, National Institute for Materials Science, Tsukuba, Ibaraki 305-0047, Japan

January 17, 2018

We present a first-principles study of $RFe_{12-x}Cr_x$ (R = Y, Nd, Sm) crystals with $ThMn_{12}$ structure in “First-principles study of intersite magnetic couplings and Curie temperature in $RFe_{12-x}Cr_x$ (R = Y, Nd, Sm)”. In this material, we offer some detailed data from our calculation: the total and local magnetic moments, average intersite magnetic interaction with wider range of the Cr concentration than the range shown in the main paper, and partial d-DOS of the Cr and Fe sites in $Sm(FeCr)_{12}$ are presented.

## 1 Magnetic moment

Figure 1 shows the total magnetic moment of $R(Fe_{12-x}Cr_x)$ and $R(Fe_{12-x}Co_x)$ (R=Y, Nd, Sm) in the unit of Bohr magneton. Note that the horizontal scale of the two panels are different. The plateau appearing in $R(Fe_{12-x}Co_x)$ in the range $1 < x < 2$ is attributable to increase of the local moment at the Fe(8f) site. Absolute values of the local moments in those systems are shown in Fig. 2. The R and Cr moments are negative, and the other moments are positive.

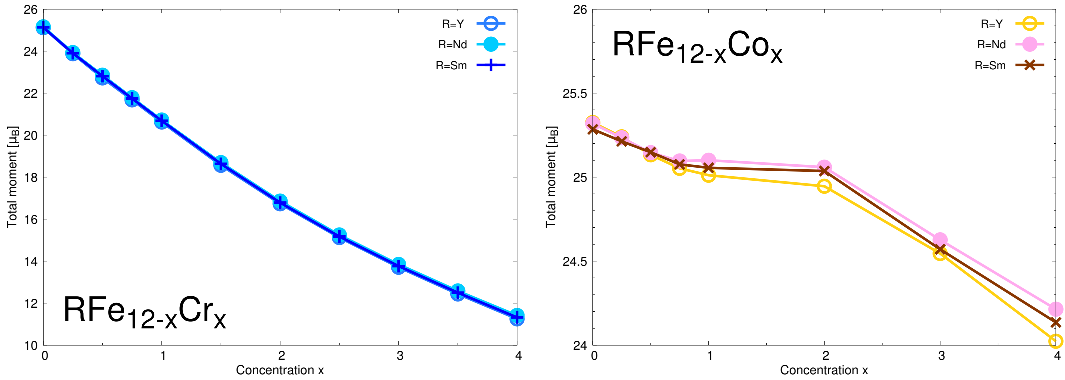


Figure 1: Total magnetic moment of $R(FeCr)_{12}$ and $R(FeCo)_{12}$ (R = Y, Nd, Sm). The contribution from the R-f electrons are excluded from the values. Note that the horizontal scales of the two panels are different from each other.

## 2 Average intersite magnetic couplings

Values of the averaged interaction in the paragraph with Eq. (5) in the main paper are shown for the range $0 \leq x \leq 4$ in Fig. 3. All values for the Cr–Cr and Fe–Cr couplings are negative, and all the others are positive.

## 3 Partial d-DOS of Cr and Fe

The particular d-DOS of the Cr and Fe sites in $Sm(Fe_{12-x}Cr_x)$ are shown in Fig. 4 for $x = 0, 0.5, 4$.

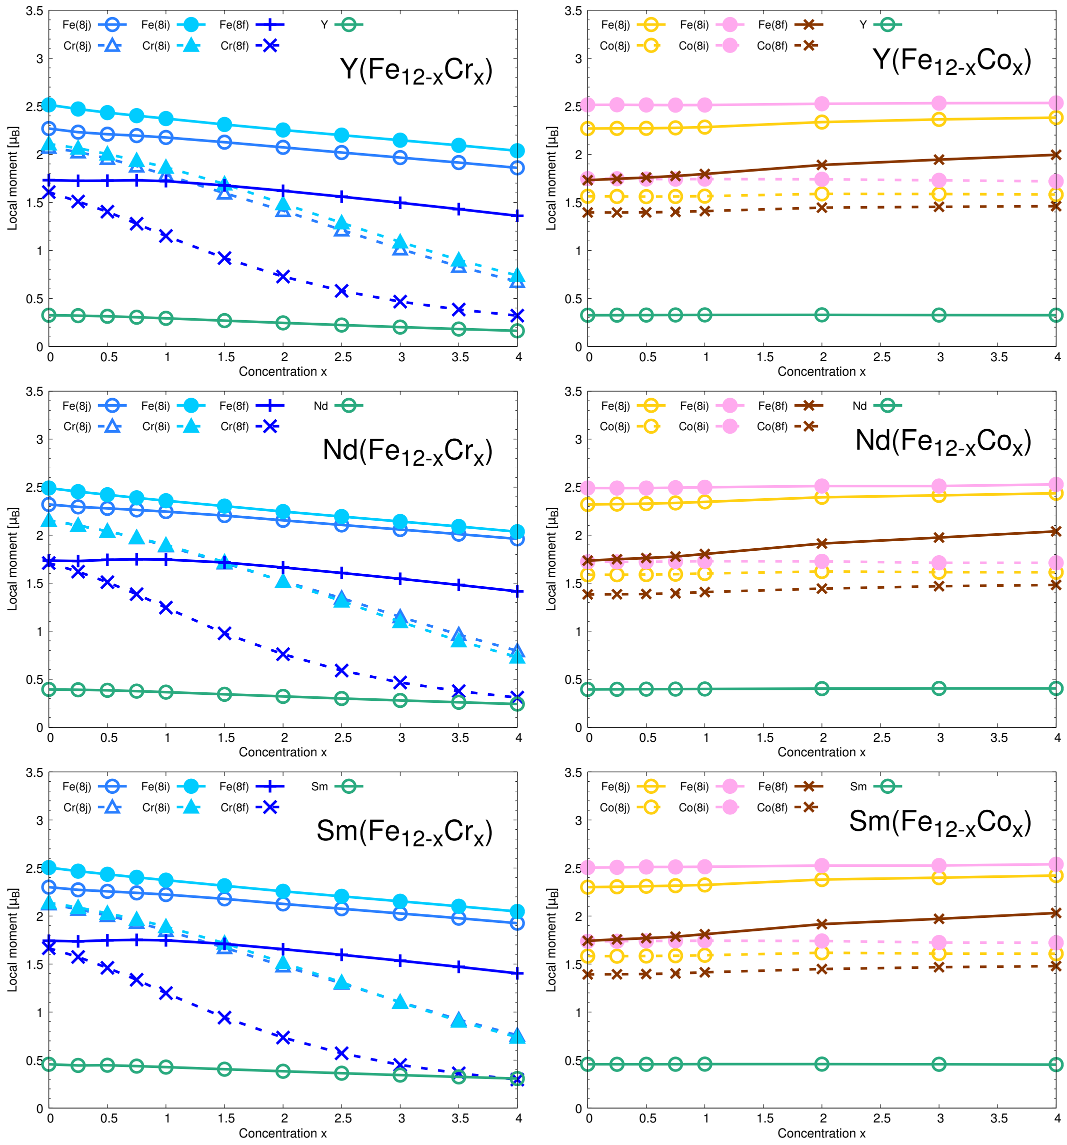


Figure 2: Absolute Values of the local moments in $R(FeCr)_{12}$ and $R(FeCo)_{12}$ (R = Y, Nd, Sm). The contribution from the R-f electrons are excluded from the values for the R elements. The moments of the Cr sites and the R sites are negative; and the others are positive.

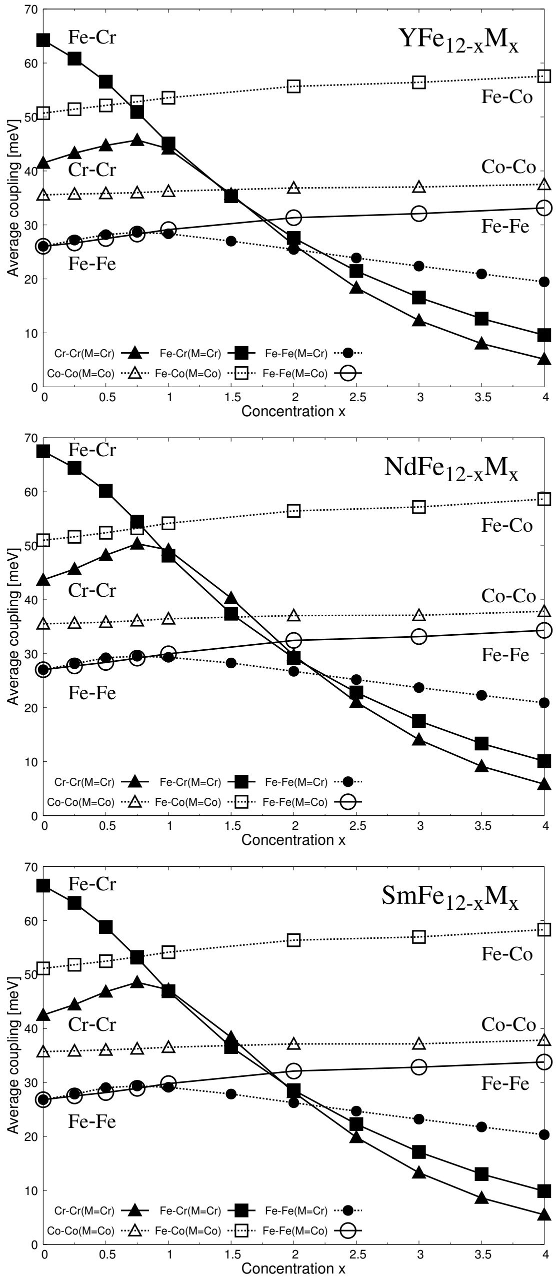


Figure 3: Absolute values of $\mathcal{J}_{\mathrm{M-M}}$, $\mathcal{J}_{\mathrm{Fe-M}}$ and $\mathcal{J}_{\mathrm{Fe-Fe}}$ [which are average of the sum defined by Eq. (5) in the main paper] in $\mathrm{RFe}_{12-x}\mathrm{M}_x$ (R=Y, Nd, Sm; M=Cr, Co) in the range $0 \leq x \leq 4$. All values of $\mathcal{J}_{\mathrm{Fe-Cr}}$ and $\mathcal{J}_{\mathrm{Cr-Cr}}$ are negative, and the other values are positive.

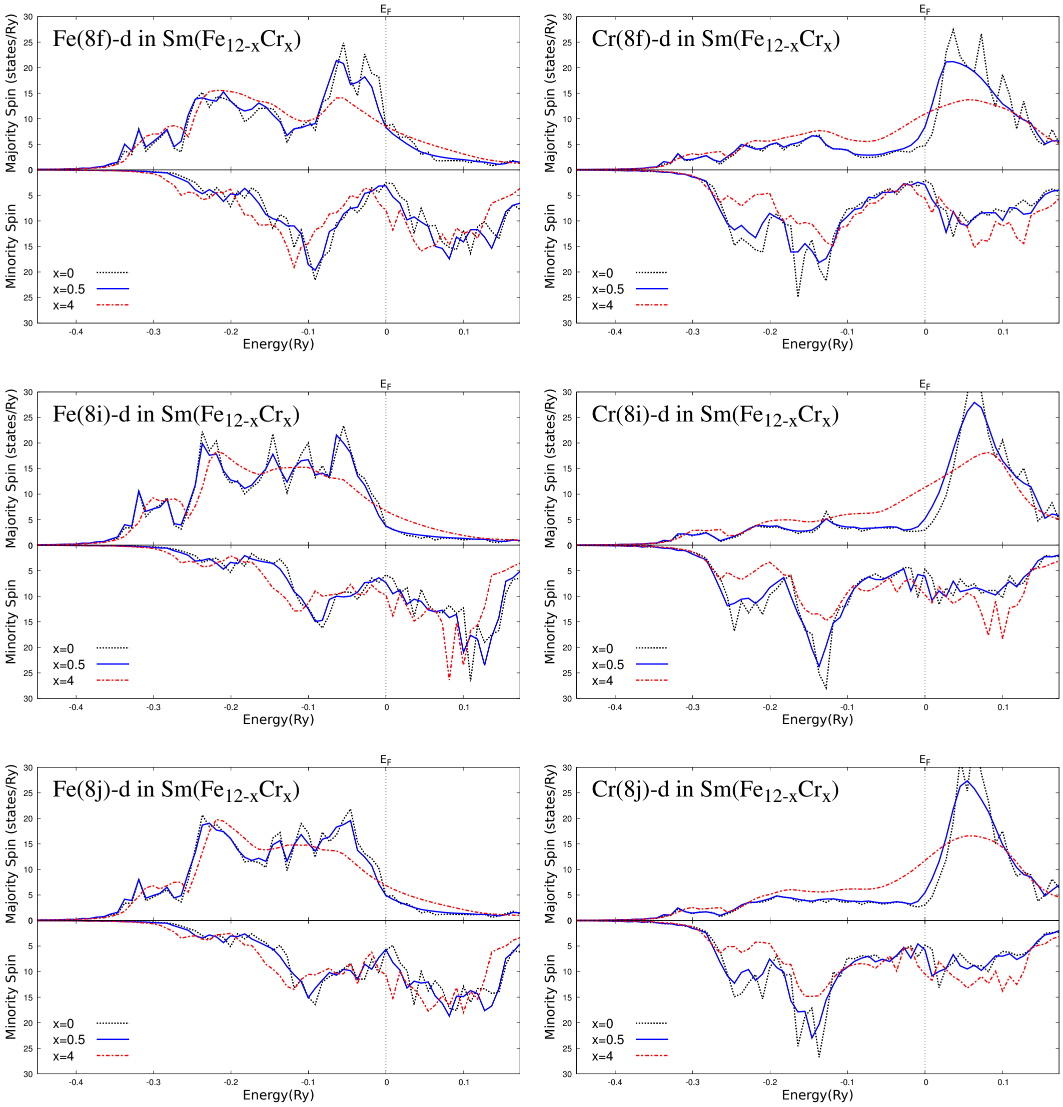


Figure 4: Partial density of states of Cr-d and Fe-d states in $Sm(Fe_{12-x}Cr_x)$ is shown for $x = 0, 0.5, 4$ with black dotted, blue solid, and red dash-dot lines, respectively.
